# Supplementary material for: Null It Out: Guarding Protected Attributes by Iterative Nullspace Projection
Source: arXiv:2004.07667 source file (2020-04-28)
Supplement: Supplementary file 1 [file appendix.tex]

% \documentclass[11pt,a4paper]{article}
% \usepackage{hyperref}
% \usepackage{xr-hyper}
% %\externaldocument{main}

% \begin{document}

\documentclass[11pt,a4paper]{article}

\usepackage[hyperref]{acl2020}
\usepackage{xr}

\usepackage{graphicx}
\usepackage{xcolor}
\definecolor{color1}{rgb}{0.4, 0., 0.} 
\definecolor{color2}{rgb}{0.6, 0.4, 1} 

\usepackage{times}
\usepackage{latexsym}
\usepackage[utf8]{inputenc}
\usepackage{xcolor}
\usepackage{linguex}
\usepackage{longtable}
\usepackage{rotating}
\usepackage{float}
\usepackage{booktabs}
\usepackage{multirow} % for the tables.
\usepackage{url}
\usepackage{hyperref}
\usepackage{amsmath}
\usepackage{amssymb}

\usepackage[ruled,vlined]{algorithm2e}
\usepackage{algorithm}
\usepackage[noend]{algpseudocode}
\usepackage{algpseudocode}
\usepackage[]{algorithm2e}
\usepackage{esvect}
\usepackage{array}
\usepackage[export]{adjustbox}

\usepackage{subfig}

\usepackage[margin=1in,headsep=.2in]{geometry}

\makeatletter
\newcommand*{\addFileDependency}[1]{% argument=file name and extension
  \typeout{(#1)}
  \@addtofilelist{#1}
  \IfFileExists{#1}{}{\typeout{No file #1.}}
}
\makeatother

% This is not strictly necessary, and may be commented out,
% but it will improve the layout of the manuscript,
% and will typically save some space.
\usepackage{microtype}

%\aclfinalcopy % Uncomment this line for the final submission
%\def\aclpaperid{***} %  Enter the acl Paper ID here

%\setlength\titlebox{5cm}
% You can expand the titlebox if you need extra space
% to show all the authors. Please do not make the titlebox
% smaller than 5cm (the original size); we will check this
% in the camera-ready version and ask you to change it back.

\usepackage{algorithm}
\usepackage{adjustbox} % resizing tables
%\pagestyle{fancy}
%\fancyhead[L,C]{}
%\lhead{Accepted as a long paper in NAACL 2019}

%\renewcommand{\firstrefdash}{}
 %  Enter the acl Paper ID here

%\newcommand{\yg}[1]{\textcolor{purple}{[YG: #1]}}
      
% \aclfinalcopy

%\title{Null It Out! Debiasing First Order Features From Decision Representations}
%\thispagestyle
% \head{}
\title{Guarding Protected Attributes by Iterative Nullspace Projection}

% \author{Shauli Ravfogel\textsuperscript{1} \;\;\; Yoav Goldberg\textsuperscript{1,2} \;\;\; Tal Linzen\textsuperscript{3} \\
% \textsuperscript{1}Computer Science Department, Bar Ilan University \\
% \textsuperscript{2}Allen Institute for Artificial Intelligence \\
% \textsuperscript{3}Department of Cognitive Science, Johns Hopkins University \\
%   {\tt \{shauli.ravfogel, yoav.goldberg\}@gmail.com, tal.linzen@jhu.edu}
%   }

%\renewcommand{\yg}[1]{}
%\renewcommand{\sr}[2]{}
%\renewcommand{\tl}[3]{}

\date{}

\begin{document}

\maketitle

% \end{document}
% \appendix
\section{Appendix}
\label{appendix}

\subsection{Most Changed Words}

In Table 1 % \ref{table:word_change}
we show the words that changed the most in average over all professions.
In Figure 1 % \ref{fig:rel-change}
we present the relative change of biased word for each profession, compared to a random sample.
\input{tables/most_changed_words.tex}
% \newpage
%\input{words-before-and-after.tex}

% \begin{table*}[t]

\\w: maiden
\\ most-similar-before: ('maidens', 'lady', 'rozen', 'slayer', 'widow', 'queen', 'alice', 'mother', 'dragon', 'metallica')\\
\\ most-similar-after: ('rozen', 'hallowed', 'maidens', 'motorhead', 'nwobhm', 'fillies', 'moonchild', 'megadeth', 'metallica', 'manowar')\\
----------------------------------
\\w: msrp
\\ most-similar-before: ('rrp', 'price', 'usd', 'retails', 'mileage', 'specs', 'sku', 'priced', 'pricing', 'polaris')\\
\\ most-similar-after: ('retails', 'rrp', 'price', 'mileage', 'priced', 'detailssee', 'usd', 'pricing', 'ltz', 'kawasaki')\\
----------------------------------
\\w: traveler
\\ most-similar-before: ('traveller', 'travelers', 'travellers', 'travel', 'adventurer', 'traveling', 'tripadvisor', 'tourist', 'destinations', 'getaway')\\
\\ most-similar-after: ('traveller', 'travelers', 'travellers', 'travel', 'vacationer', 'adventurer', 'traveling', 'holidaymaker', 'fareed', 'destinations')\\
----------------------------------
\\w: cast
\\ most-similar-before: ('casting', 'casts', 'actors', 'starring', 'actor', 'stars', 'star', 'iron', 'film', 'movie')\\
\\ most-similar-after: ('casting', 'aspersions', 'casted', 'casts', 'castings', 'actors', 'starring', 'svaka', 'ductile', 'enameled')\\
----------------------------------
\\w: droid
\\ most-similar-before: ('razr', 'htc', 'nexus', 'motorola', 'android', 'xoom', 'galaxy', 'smartphone', 'atrix', 'iphone')\\
\\ most-similar-after: ('htc', 'eris', 'razr', 'nexus', 'atrix', 'xoom', 'motorola', 'android', 'cliq', 'galaxy')\\
----------------------------------
\\w: hath
\\ most-similar-before: ('thou', 'hast', 'thy', 'unto', 'thee', 'doth', 'ye', 'shalt', 'behold', 'thine')\\
\\ most-similar-after: ('thee', 'thou', 'thy', 'hast', 'unto', 'shalt', 'shall', 'ye', 'thine', 'behold')\\
----------------------------------
\\w: nodes
\\ most-similar-before: ('node', 'lymph', 'configured', 'subset', 'cluster', 'corresponding', 'clusters', 'vertices', 'compute', 'configuration')\\
\\ most-similar-after: ('node', 'lymph', 'vertices', 'multicast', 'topology', 'plurality', 'routing', 'interconnected', 'routers', 'servers')\\
----------------------------------
\\w: mart
\\ most-similar-before: ('wal', 'walmart', 'stores', 'store', 'mall', 'grocery', 'depot', 'supermarket', 'costco', 'shopping')\\
\\ most-similar-after: ('wal', 'walmart', 'mall', 'marts', 'supercenter', 'stores', 'plaza', 'store', 'kmart', 'expo')\\
----------------------------------
\\w: dell
\\ most-similar-before: ('inspiron', 'hp', 'laptop', 'compaq', 'toshiba', 'lenovo', 'acer', 'vostro', 'ibm', 'notebook')\\
\\ most-similar-after: ('inspiron', 'compaq', 'vostro', 'lenovo', 'laptop', 'hp', 'poweredge', 'hewlett', 'optiplex', 'toshiba')\\
----------------------------------
\\w: uses
\\ most-similar-before: ('use', 'using', 'utilizes', 'used', 'does', 'example', 'which', 'works', 'also', 'takes')\\
\\ most-similar-after: ('utilizes', 'use', 'employs', 'utilises', 'using', 'incorporates', 'used', 'relies', 'implements', 'misuses')\\
----------------------------------
\\w: africa
\\ most-similar-before: ('african', 'kenya', 'asia', 'south', 'tanzania', 'zimbabwe', 'ghana', 'australia', 'europe', 'namibia')\\
\\ most-similar-after: ('african', 'kenya', 'namibia', 'tanzania', 'mozambique', 'continent', 'south', 'zambia', 'ghana', 'zimbabwe')\\
----------------------------------
\\w: tx
\\ most-similar-before: ('texas', 'houston', 'austin', 'dallas', 'plano', 'az', 'lubbock', 'arlington', 'tn', 'antonio')\\
\\ most-similar-after: ('texas', 'lewisville', 'dallas', 'austin', 'waco', 'houston', 'coppell', 'abilene', 'weslaco', 'antonio')\\
----------------------------------
\\w: attain
\\ most-similar-before: ('attaining', 'achieve', 'attained', 'achieving', 'accomplish', 'obtain', 'acheive', 'achieved', 'strive', 'possess')\\
\\ most-similar-after: ('attaining', 'achieve', 'attained', 'achieving', 'acheive', 'accomplish', 'attainable', 'attains', 'accomplishing', 'attainment')\\
----------------------------------
\\w: du
\\ most-similar-before: ('le', 'des', 'au', 'dans', 'de', 'les', 'à', 'monde', 'sur', 'pont')\\
\\ most-similar-after: ('des', 'le', 'au', 'sur', 'monde', 'avec', 'cinéma', 'toit', 'pont', 'soleil')\\
----------------------------------
\\w: nice
\\ most-similar-before: ('good', 'lovely', 'very', 'awesome', 'great', 'pretty', 'really', 'wonderful', 'fantastic', 'excellent')\\
\\ most-similar-after: ('lovely', 'very', 'good', 'amvery', 'nicely', 'pmnice', 'really', 'neat', 'pleasant', 'well')\\
----------------------------------
\\w: elliot
\\ most-similar-before: ('elliott', 'todd', 'stuart', 'russell', 'cohen', 'eliot', 'randall', 'bennett', 'ross', 'gould')\\
\\ most-similar-after: ('elliott', 'yamin', 'missy', 'denholm', 'eliot', 'sadler', 'eliott', 'gardiner', 'aronson', 'fibonacci')\\
----------------------------------
\\w: oprah
\\ most-similar-before: ('winfrey', 'degeneres', 'palin', 'celebrity', 'leno', 'tyra', 'letterman', 'beyonce', 'interview', 'cnn')\\
\\ most-similar-after: ('winfrey', 'degeneres', 'leno', 'harpo', 'nightline', 'tyra', 'limbaugh', 'hannity', 'couric', 'reelzchannel')\\
----------------------------------
\\w: pierre
\\ most-similar-before: ('georges', 'francois', 'michel', 'laurent', 'jacques', 'antoine', 'françois', 'jean', 'henri', 'yves')\\
\\ most-similar-after: ('bourdieu', 'francois', 'françois', 'georges', 'chardin', 'yves', 'antoine', 'laurent', 'miquelon', 'christophe')\\
----------------------------------
\\w: censorship
\\ most-similar-before: ('censors', 'censor', 'censoring', 'criticism', 'neutrality', 'piracy', 'repression', 'sopa', 'draconian', 'activism')\\
\\ most-similar-after: ('censors', 'censor', 'censoring', 'repression', 'sopa', 'circumvention', 'protest', 'clampdown', 'blacklisting', 'imposed')\\
----------------------------------
\\w: hampshire
\\ most-similar-before: ('nh', 'massachusetts', 'vermont', 'maine', 'connecticut', 'rhode', 'delaware', 'portsmouth', 'pennsylvania', 'virginia')\\
\\ most-similar-after: ('nh', 'massachusetts', 'maine', 'vermont', 'connecticut', 'nashua', 'rhode', 'waterlooville', 'seacoast', 'lymington')\\
----------------------------------
\\w: protection
\\ most-similar-before: ('protect', 'protective', 'protecting', 'protected', 'safety', 'security', 'protects', 'shield', 'safeguard', 'prevention')\\
\\ most-similar-after: ('protect', 'protects', 'protecting', 'protective', 'safeguard', 'protector', 'protected', 'protections', 'shield', 'shields')\\
----------------------------------
\\w: meats
\\ most-similar-before: ('meat', 'cheeses', 'vegetables', 'sausages', 'foods', 'beef', 'steaks', 'pork', 'salads', 'veggies')\\
\\ most-similar-after: ('meat', 'cheeses', 'vegetables', 'foods', 'sausages', 'beef', 'steaks', 'salads', 'grilled', 'seafood')\\
----------------------------------
\\w: instead
\\ most-similar-before: ('rather', 'either', 'then', 'simply', 'while', 'basically', 'just', 'because', 'actually', 'them')\\
\\ most-similar-after: ('rather', 'substituting', 'basically', 'opposed', 'trying', 'essentially', 'adding', 'insted', 'while', 'try')\\
----------------------------------
\\w: auckland
\\ most-similar-before: ('christchurch', 'sydney', 'melbourne', 'zealand', 'wellington', 'brisbane', 'adelaide', 'dunedin', 'perth', 'canberra')\\
\\ most-similar-after: ('sydney', 'christchurch', 'melbourne', 'invercargill', 'tauranga', 'zealand', 'adelaide', 'nz', 'rotorua', 'manukau')\\
% \newpage
% \end{table*}

\begin{figure}[]
    \centering
    \includegraphics[width=1.0\columnwidth]{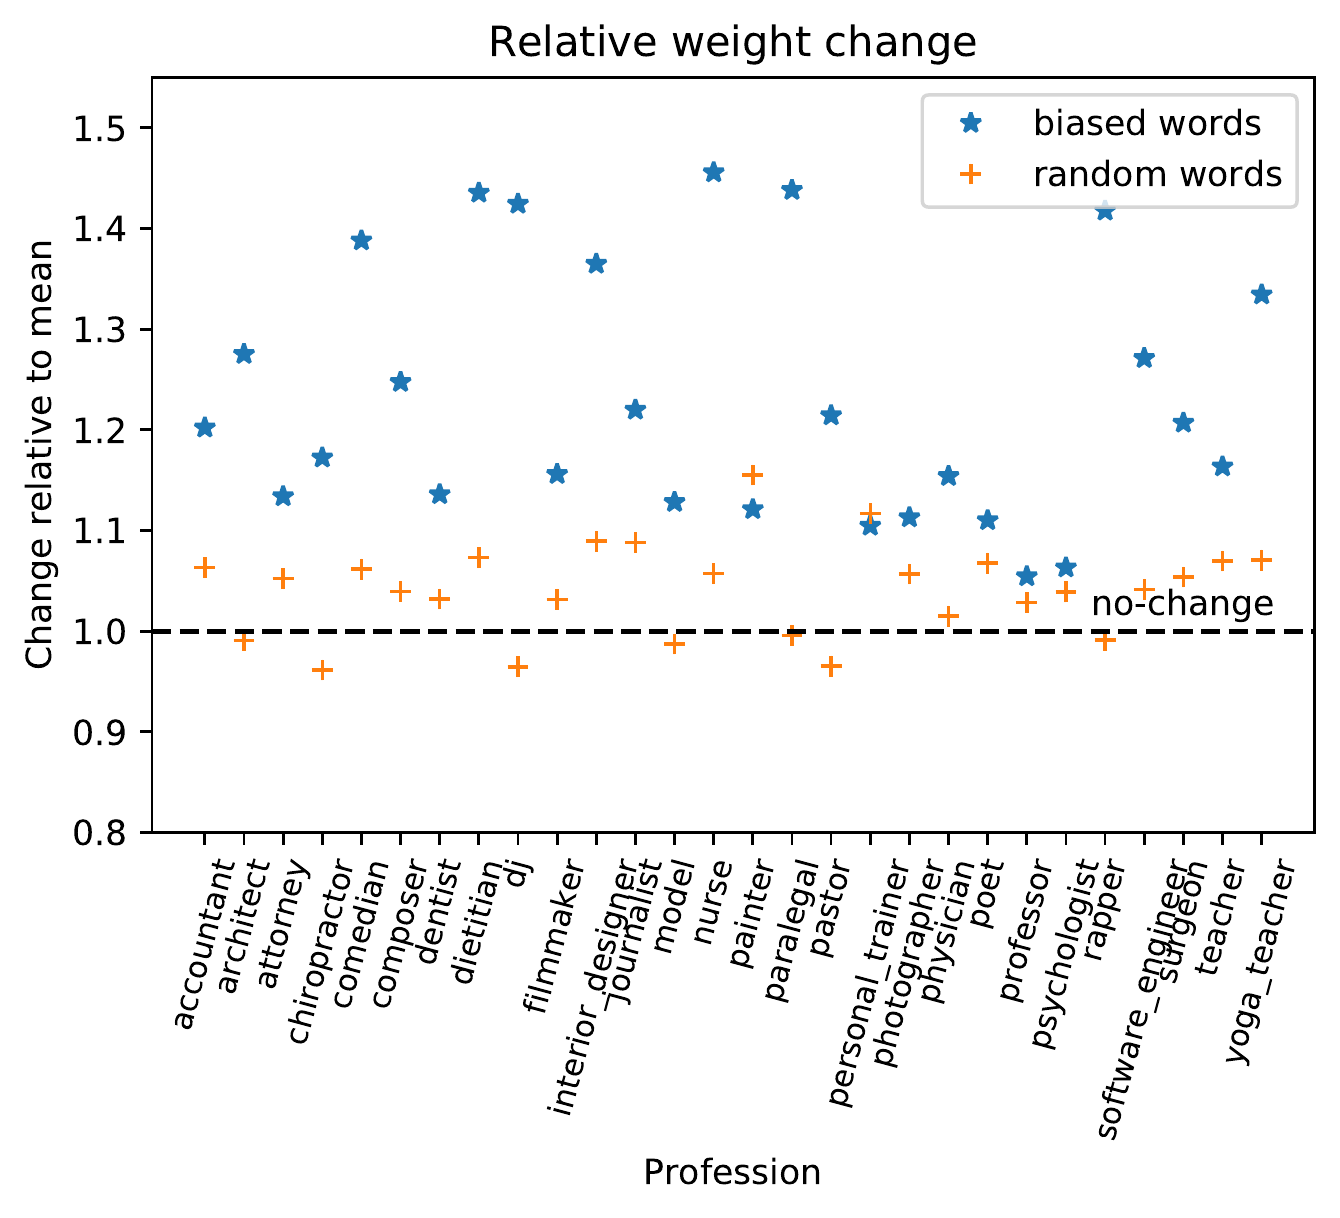}
    \caption{The relative change of biased vs. random words, per profession. }
    \label{fig:rel-change}
\end{figure}

\newpage

\subsection{Closest Glove Vectors Before and After the Projection}
\label{neighbors-examples}
In Table 2, %\ref{table:nearest_words},
we show the top 3-nearest neighbors of sampled words from GloVe, before and after the INLP process.

\newpage
\newpage

% \begin{figure*}[t!]
%     \centering
%     \includegraphics[scale=0.045]{plots/word2vec-debiasing-progress.png}
%     \caption{T-SNE projection of GLoVE vectors of the most biased words after 0, 5, 18 and 35 iterations of INLP.}
%     \label{fig:tsne}
    
% \end{figure*}

\end{document}
